# Supplementary material for: NIFTY: Neural Object Interaction Fields for Guided Human Motion Synthesis
Source: arXiv:2307.07511 source file (2023-07-14)
Supplement: Supplementary file 1 [file overview.tex]

\section{Overview}

This supplementary material provides additional context on the details of the paper along with supplemental results that were omitted due to space constraints. 
In addition to this document (\texttt{supplementary.pdf}), we also provide an HTML webpage of video results (\texttt{supplementary.html}) and \texttt{supp\_video\_source} contains all the videos in the webpage. 
\textbf{We encourage the reader to view the webpage} of qualitative results and data examples, which are best to judge the quality of motion and compare results. 
% Below we discuss the overview of the rest of the supplementary in the following sections.

In \S \ref{sec:datagen}, we discuss additional details of our data collection algorithm and evaluate data quality with a user study, while \S \ref{sec:implementation} provides details of our \ours model.  \S \ref{sec:qualitative} discusses additional qualitative results. In \S\ref{sec:quantitative}, we provide additional details on experiments from the main paper, including our baseline comparison user study in \S\ref{subsec:userstudy} and the behavior of different metrics.
\S \ref{sec:newresults} provides supplemental results to further analyze the performance of our diffusion model and interaction field. 
Finally, \S \ref{sec:failures} discusses limitations.
