# Supplementary material for: NIFTY: Neural Object Interaction Fields for Guided Human Motion Synthesis
Source: arXiv:2307.07511 source file (2023-07-14)
Supplement: Supplementary file 2 [file baseline.tex]

\begin{table}[h!]
    \setlength{\tabcolsep}{3pt}
    \caption{\textbf{Baseline Full Metrics.} } 
    \centering 
    \vspace{-1mm}
    \begin{adjustbox}{max width=\linewidth}
    
     \begin{tabular}{l r@{~~}r@{~~}rr@{~~}rrr} \toprule
        
                & \multicolumn{7}{r}{\textbf{Sitting}} \\
                % \midrule
        Method  & Foot                 & \% {\it D2O}          &  {\it D2O}                              & Skel.                &  \% Skel.                   & Contact               & \% Pen.  \\
                & Skating $\downarrow$ & $\le 2cm$ $\uparrow$  &  $95^\text{th}\tilde{\%}$ $\downarrow$  & Dist. $\downarrow$   & Dist.$\le 25cm$ $\uparrow$ & IoU    $\uparrow$     &  $\le 2cm$ $\uparrow$   \\
                 \midrule   
         \humanise  & 0.77 & 88.84 & 0.13 & 1.07 & 2.59 & 0.21 & 46.41\\
         \mdmOnly & 0.36 & 37.85 & 1.06 & 2.81 & 0.00 & 0.04 & 50.00 \\
         \ours (ours) & 0.47 & 99.60 & 0.00 & 0.54 & 65.94 & 0.54 & 65.40 \\
        
    \end{tabular}
    \end{adjustbox}
    
    \begin{adjustbox}{max width=\linewidth}
    
     \begin{tabular}{l s@{~~}s@{~~}ss@{~~}sss} \toprule
        
                & \multicolumn{7}{s}{\textbf{Lifting}} \\
                % \midrule
        Method  & Foot                 & \% {\it D2O}          &  {\it D2O}                              & Skel.                &  \% Skel.                   & Contact               & \% Pen.  \\
                & Skating $\downarrow$ & $\le 2cm$ $\uparrow$  &  $95^\text{th}\tilde{\%}$ $\downarrow$  & Dist. $\downarrow$   & Dist.$\le 25cm$ $\uparrow$ & IoU    $\uparrow$     &  $\le 2cm$ $\uparrow$   \\
                 \midrule
         \humanise  & 0.66 & 57.37 & 0.66 & 1.70 & 1.39 & 0.03 & 61.11\\
         \mdmOnly & 0.28 & 36.26 & 1.14 & 2.58 & 1.00 & 0.02 & 45.05 \\
        \ours (ours)  & 0.34 & 77.69 & 0.05 & 0.42 & 61.55 & 0.17 & 69.49 \\
        \midrule
    \end{tabular}
    \end{adjustbox}

    \label{tab:baseline_extra}
   
\end{table}
