# Supplementary material for: NIFTY: Neural Object Interaction Fields for Guided Human Motion Synthesis
Source: arXiv:2307.07511 source file (2023-07-14)
Supplement: Supplementary file 3 [file extra.tex]

Add extra sentences of supp here.
