# Supplementary material for: NIFTY: Neural Object Interaction Fields for Guided Human Motion Synthesis
Source: arXiv:2307.07511 source file (2023-07-14)
Supplement: Supplementary file 4 [file tmp-pdfcrop-6275.tex]

\catcode37 14 % percent
\catcode33 12 % exclam
\catcode34 12 % quote
\catcode35  6 % hash
\catcode39 12 % apostrophe
\catcode40 12 % left parenthesis
\catcode41 12 % right parenthesis
\catcode45 12 % minus
\catcode46 12 % period
\catcode60 12 % less
\catcode61 12 % equals
\catcode62 12 % greater
\catcode64 12 % at
\catcode91 12 % left square
\catcode93 12 % right square
\catcode96 12 % back tick
\catcode123 1 % left curly brace
\catcode125 2 % right curly brace
\catcode126 12 % tilde
\catcode`\#=6 %
\escapechar=92 %
\def\IfUndefined#1#2#3{%
  \begingroup\expandafter\expandafter\expandafter\endgroup
  \expandafter\ifx\csname#1\endcsname\relax
    #2%
  \else
    #3%
  \fi
}
\def\pdffilehex{6C696B6572745F757365725F696E737472756374696F6E732E706466}
\IfUndefined{pdfunescapehex}{%
  \begingroup
    \gdef\pdffile{}%
    \def\do#1#2{%
      \ifx\relax#2\relax
        \ifx\relax#1\relax
        \else
          \errmessage{Invalid hex string, should not happen!}%
        \fi
      \else
        \lccode`0="#1#2\relax
        \lowercase{%
          \xdef\pdffile{\pdffile0}%
        }%
        \expandafter\do
      \fi
    }%
    \expandafter\do\pdffilehex\relax\relax
  \endgroup
}{%
  \edef\pdffile{\pdfunescapehex{\pdffilehex}}%
}
\immediate\write-1{Input file: \pdffile}
\pdfcompresslevel=9  \pdfoutput=1 %
\csname pdfmapfile\endcsname{}
\def\setpdfversion#1#2{%
  \IfUndefined{pdfobjcompresslevel}{%
  }{%
    \ifnum#1=1 %
     \ifnum#2<5
       \pdfobjcompresslevel=0 %
     \else
       \pdfobjcompresslevel=2 %
     \fi
   \fi 
  }%
  \IfUndefined{pdfminorversion}{%
    \IfUndefined{pdfoptionpdfminorversion}{%
    }{%
      \pdfoptionpdfminorversion=#2\relax
    }%
  }{%
    \pdfminorversion=#2\relax
    \IfUndefined{pdfmajorversion}{%
      \ifnum#2=0 \pdfminorversion=5\fi}
      {\pdfmajorversion=#1\relax}%
  }%
}
\def\page #1 [#2 #3 #4 #5]{%
  \count0=#1\relax
  \setbox0=\hbox{%
    \pdfximage page #1 mediabox{\pdffile}%
    \pdfrefximage\pdflastximage
  }%
  \pdfhorigin=-#2bp\relax
  \pdfvorigin=#3bp\relax
  \pdfpagewidth=#4bp\relax
  \advance\pdfpagewidth by -#2bp\relax
  \pdfpageheight=#5bp\relax
  \advance\pdfpageheight by -#3bp\relax
  \ht0=\pdfpageheight
  \shipout\box0\relax
}
\def\pageclip #1 [#2 #3 #4 #5][#6 #7 #8 #9]{%
  \count0=#1\relax
  \dimen0=#4bp\relax \advance\dimen0 by -#2bp\relax
  \edef\imagewidth{\the\dimen0}%
  \dimen0=#5bp\relax \advance\dimen0 by -#3bp\relax
  \edef\imageheight{\the\dimen0}%
  \pdfximage page #1 mediabox{\pdffile}%
  \setbox0=\hbox{%
    \kern -#2bp\relax
    \lower #3bp\hbox{\pdfrefximage\pdflastximage}%
  }%
  \wd0=\imagewidth\relax
  \ht0=\imageheight\relax
  \dp0=0pt\relax
  \pdfhorigin=#6pt\relax
  \pdfvorigin=#7bp\relax
  \pdfpagewidth=\imagewidth
  \advance\pdfpagewidth by #6bp\relax
  \advance\pdfpagewidth by #8bp\relax
  \pdfpageheight=\imageheight\relax
  \advance\pdfpageheight by #7bp\relax
  \advance\pdfpageheight by #9bp\relax
  \pdfxform0\relax
  \shipout\hbox{\pdfrefxform\pdflastxform}%
}%
\def\pageinclude#1{%
  \pdfhorigin=0pt\relax
  \pdfvorigin=0pt\relax
  \pdfximage page #1 mediabox{\pdffile}%
  \setbox0=\hbox{\pdfrefximage\pdflastximage}%
  \pdfpagewidth=\wd0\relax
  \pdfpageheight=\ht0\relax
  \advance\pdfpageheight by \dp0\relax
  \shipout\hbox{%
    \raise\dp0\box0\relax
  }%
}
\setpdfversion{1}{3}
