# Supplementary material for: NIFTY: Neural Object Interaction Fields for Guided Human Motion Synthesis
Source: arXiv:2307.07511 source file (2023-07-14)
Supplement: Supplementary file 5 [file todo.tex]

\begin{itemize}
  \item Writing
    \begin{itemize}
        \item 
    \end{itemize}
  \item Videos
  \item Ablations \& Results
  
\end{itemize}
